# Supplementary material for: Convex Hierarchical Clustering for Graph-Structured Data
Source: arXiv:1911.03417 source file (2019-12-11)
Supplement: Supplementary file 1 [file appendix_scalable.tex]

% !TEX root = HC_nips_2018.tex

We here detail an extension of the algorithm to make it scalable to much larger matrices.Indeed, the information contained  in $\pi$ is redundant as some clusters are repeated. Hence what we would like to do is keep the information in a matrix  keeping track of the coalescent paths between the clusters.
This being said, we start with the observation that the matrix $\pi$ can be factorized as follows:
$$ \pi = W E, \quad W \in \R^{N \times K}, E \in \R^{K \times N}$$

where $W$ is the doubly-stochastic matrix corresponding to the assignment of each observation $i$ to the $K$ clusters, while $E$ is a cluster coalescence matrix:
\[E_{kj} = \begin{cases}
1 \text{ if   centroid $j$ is in cluster $k$}\\
0 \text{ otherwise}
\end{cases}\]
$E$ is thus a hard assignment matrix showing which clusters have coalesced with which and:
$$ \pt k,j \in [1,K]\times [1,N], \quad  E_{kj} \in \{0,1\}, \text{ and } \sum_{k=1}^K E_{kj}=1$$
This would help the storage bottle neck since the algorithm would only require the storage of $2 K \times N$ matrices (instead of the $N\times N$ matrices that it previously had to store.)
The previous optimization problem can thus be re-written as:
$$       \text{arg min }_{W \in \Delta_{N,K}, E \in \tilde{\Delta}_{K,N}} \text{Trace} [ E^TW^T K WE  -2 K  WE \Big] +2\lambda \sum_{i,j}K_{ij}\text{Pen}\Big(E_{i} -E_{ j}\Big)\\$$
where $\Delta_{N,K}$ is the set of doubly-stochastic matrices in $\R^{N \times K}$ and $\tilde{\Delta}_{K,N}$ is the set of column-wise stochastic matrices in $\R^{K \times N}$. \\

We begin by making the following observations:
\begin{itemize}
\item  The problem is no longer jointly convex in $E$ and $W$, but bi-convex.
\item The penalty is only carried by the matrix $E$: indeed, the different $K$ clusters are a priori-unknown and the way they are attributed is penalty-free. However, the centroids corresponding to 
\item We can relax the assumption that $E$ is $\{0,1\}$ valued to make our lives simpler and simply assume that $E$ is a column-wise stochastic matrix. Note that that we prefer this relaxation in lieu of the traditional $E E^T=I$that is typically demanded in spectral clustering, because we typically want to allow the points to spread in less clusters than the $K$ that are already available.
\item Our solving procedure will thus alternate between solving for $E$ and solving for $W$ calmly.
\end{itemize}

\subsubsection{Solving for $W$}

In this setting, we assume that the matrix $E$ is given and we attempt to solve for $W$.
Using the permutation invariance properties of the trace, the optimization problem in terms of $W$ boils down to:
$$       \text{arg min }_{W \in \Delta_{N,K}} \text{Trace} [ W^T K WEE^T  -2 K  WE \Big] \\$$
Now, the gradient of the previous objective is given by:
$$\nabla_W \mathcal{L}(W,E)= K^T W (EE^T)^T+ K W (EE^T)-2KE^T= 2K W (EE^T)-2KE^T$$
Hence, this gradient is Lipschitz, with Lipschitz constant:
$$||\nabla_W \mathcal{L}(W_1,E) -\nabla_W \mathcal{L}(W_2,E)||_F^2 = 4 || K (W_1-W_2) EE^T||_F^2 \leq  4   ||K||_F^2 || EE^T||^2  ||W_1-W_2||_F^2 $$

where $|| \cdot||$ is the operator norm $||K||^2 =\sup_{||x||=1}||Kx||^2=\sup_{||x||=1}  \sum_{i,j} (K_{ij}x_j)^2 \leq  N \max(K)$
Hence we can apply the fast Projected Gradient descent algorithm to solve for $W$.  
\subsubsection{Solving for $E$}
The problem in $E$ is a little less simple, as it includes all the coupling constraints.
Here, we assume that $W$ is fixed, and the problem thus boils down to solving:
$$       \text{arg min }_{E \in \tilde{\Delta}_{K,N}} \text{Trace} [ E^TW^T K WE  -2 K  WE \Big] \\$$
which is essentially the same problem as we had in the first part, except that now $E$ is simply stochastic (instead of doubly stochastic).
