# Supplementary material for: Convex Hierarchical Clustering for Graph-Structured Data
Source: arXiv:1911.03417 source file (2019-12-11)
Supplement: Supplementary file 2 [file appendix_FGD.tex]

% !TEX root = HC_nips_2018.tex

We here provide a little background information on the Fast Projected Gradient Descent Algorithm that is used throughout the paper at various instances.
